# Supplementary material for: Ab-Initio Molecular Dynamics with Screened Lorentz Forces. Part II. Efficient Propagators and Rovibrational Spectra in Strong Magnetic Fields
Source: arXiv:2105.04225 source file (2021-05-10)
Supplement: Supplementary file 1 [file si.pdf]

**Supporting Information:**

**Ab-Initio Molecular Dynamics with Screened Lorentz Forces. Part II. Efficient Propagators and Rovibrational Spectra in Strong Magnetic Fields**

Laurens D. M. Peters,[1, a)] Tanner Culpitt,[1] Laurenz Monzel,[1, 2] Erik I. Tellgren,[1] and Trygve Helgaker[1]

[1)] *Hylleraas Centre for Quantum Molecular Sciences, Department of Chemistry, University of Oslo, P.O. Box 1033 Blindern, N-0315 Oslo, Norway*

[2)] *Karlsruhe Institute of Technology (KIT), Institute of Physical Chemistry, KIT Campus South, P.O. Box 6980, D-76049 Karlsruhe, Germany*

(Dated: 7 May 2021)

[a)] Electronic mail: laurens.peters@kjemi.uio.no

CONTENTS


I. Potential Energy Surfaces 3

II. Comparison of Integration Schemes 5

III. Screening of $\omega$ 7

IV. Screening of Propagators 9

V. Screening of $\omega$ and Propagators 10

VI. Trajectories and "Translational" Spectra of He 11

VII. Trajectories of $H_2$ 12

VIII. Rovibrational Spectra of $H_2$ 13

IX. Pseudocode for Propagators 14

X. Coefficients for Propagators 15

References 17

# I. POTENTIAL ENERGY SURFACES

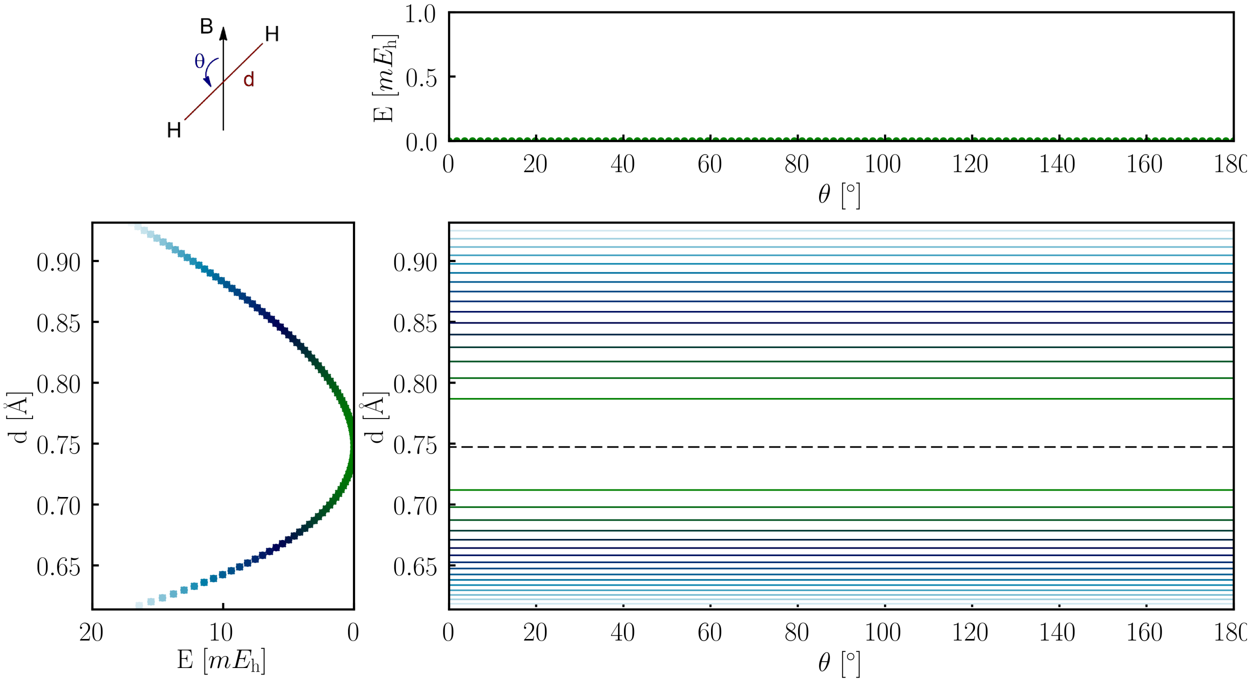


FIG. S1: Potential energy surface of $H_2$ calculated at HF/cc-pVDZ level of theory in the absence of a magnetic field. The coordinates $d$ and $\theta$ are defined in the upper left part of the figure. The dashed line indicates the minimum energy rotation.

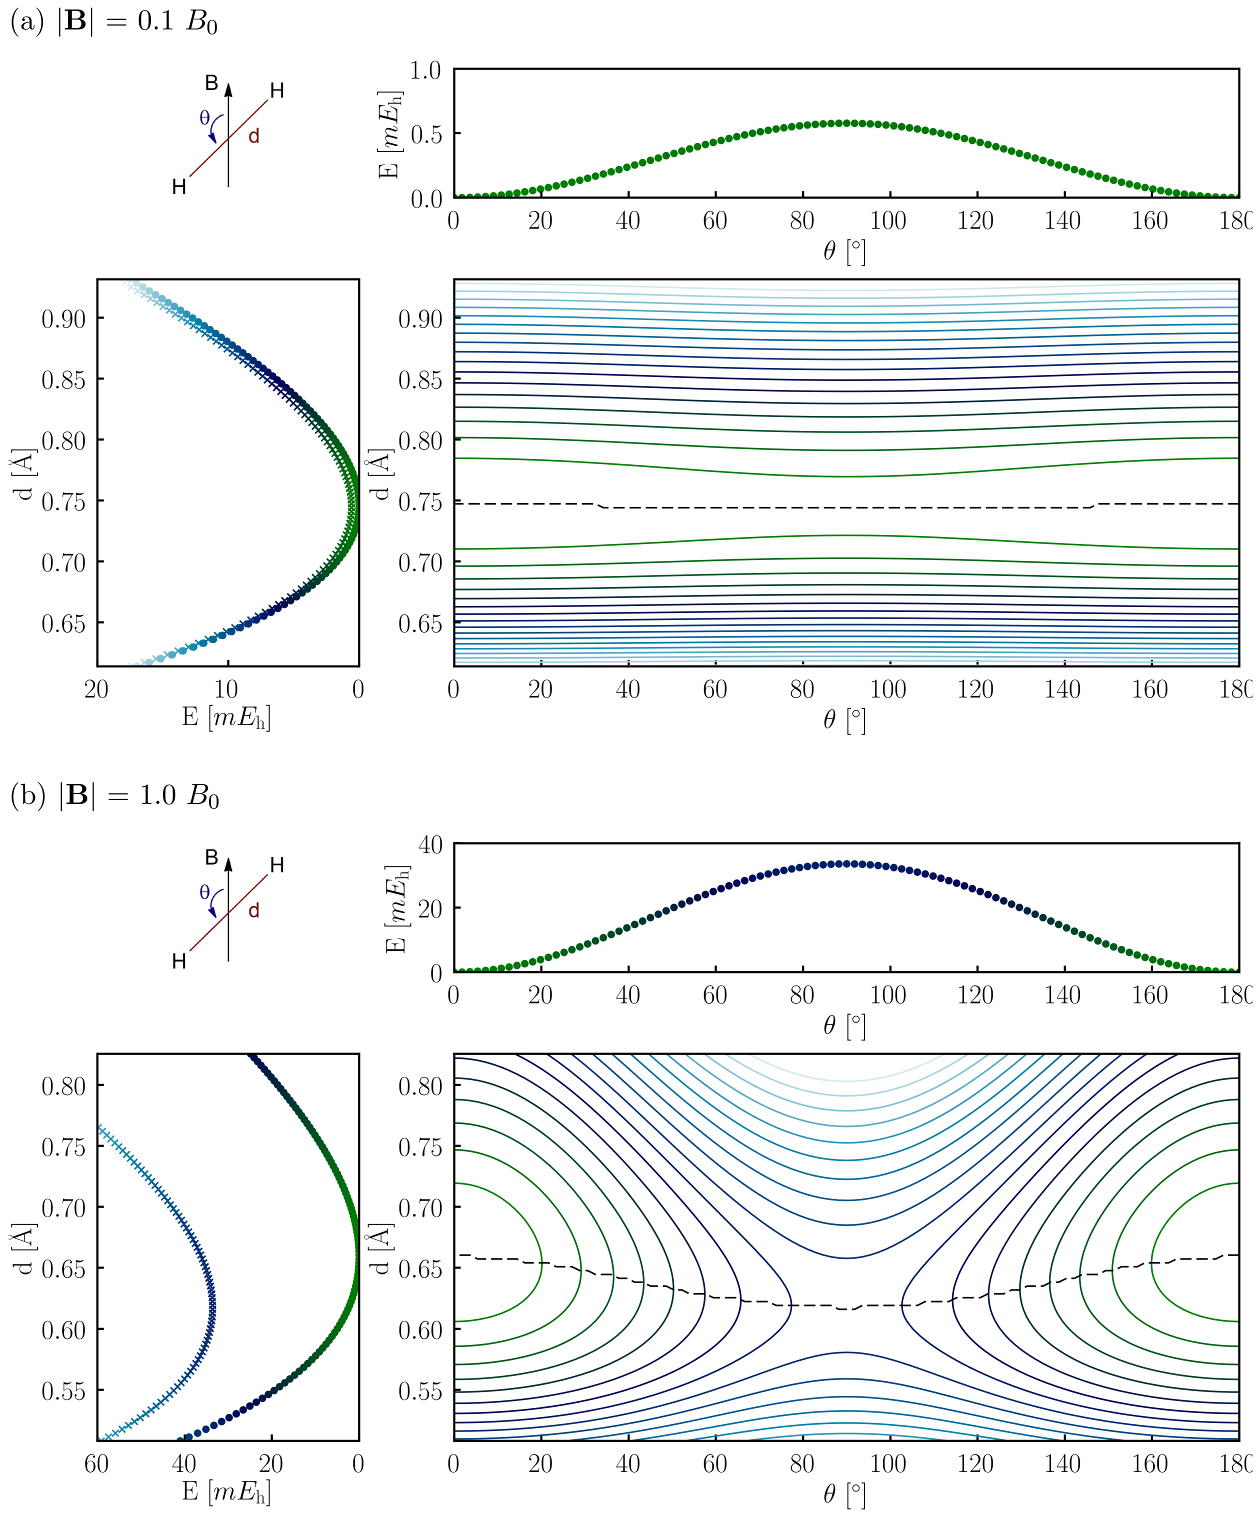


FIG. S2: Potential energy surface of $H_2$ calculated at HF/cc-pVDZ level of theory applying $|\mathbf{B}| = 0.1\ B_0$ (a) and $|\mathbf{B}| = 1.0\ B_0$ (b). The coordinates $d$ and $\theta$ are defined in the upper left part of the figure. The dashed line indicates the minimum energy rotation.

## II. COMPARISON OF INTEGRATION SCHEMES

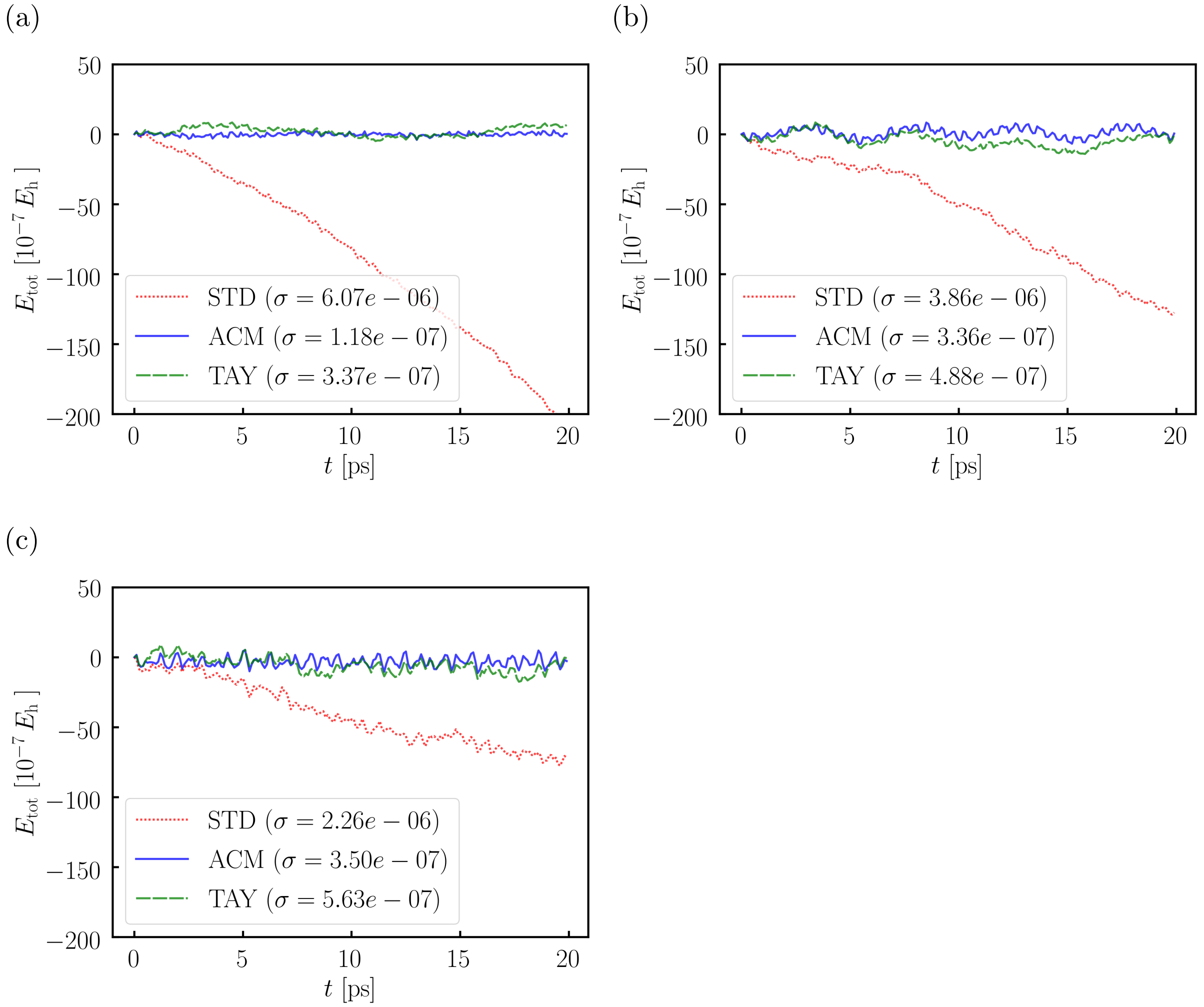


FIG. S3: Comparison of integration schemes for three trajectories (a-c) of $H_2$ (HF/cc-pVDZ level of theory, $\Delta t = 0.02\,\mathrm{fs}$, $T \approx 1000\,\mathrm{K}$) with $|\mathbf{B}| = 0.1\,B_0$: Velocity Verlet in its standard implementation (STD), auxiliary coordinates (ACM) and momenta form setting $\omega$ to 0.1, and Taylor expansion form (TAY). In all simulations, the Berry force was neglected. The standard deviation ($\sigma$) of the total energy ($E_{\mathrm{tot}}$) is also given.

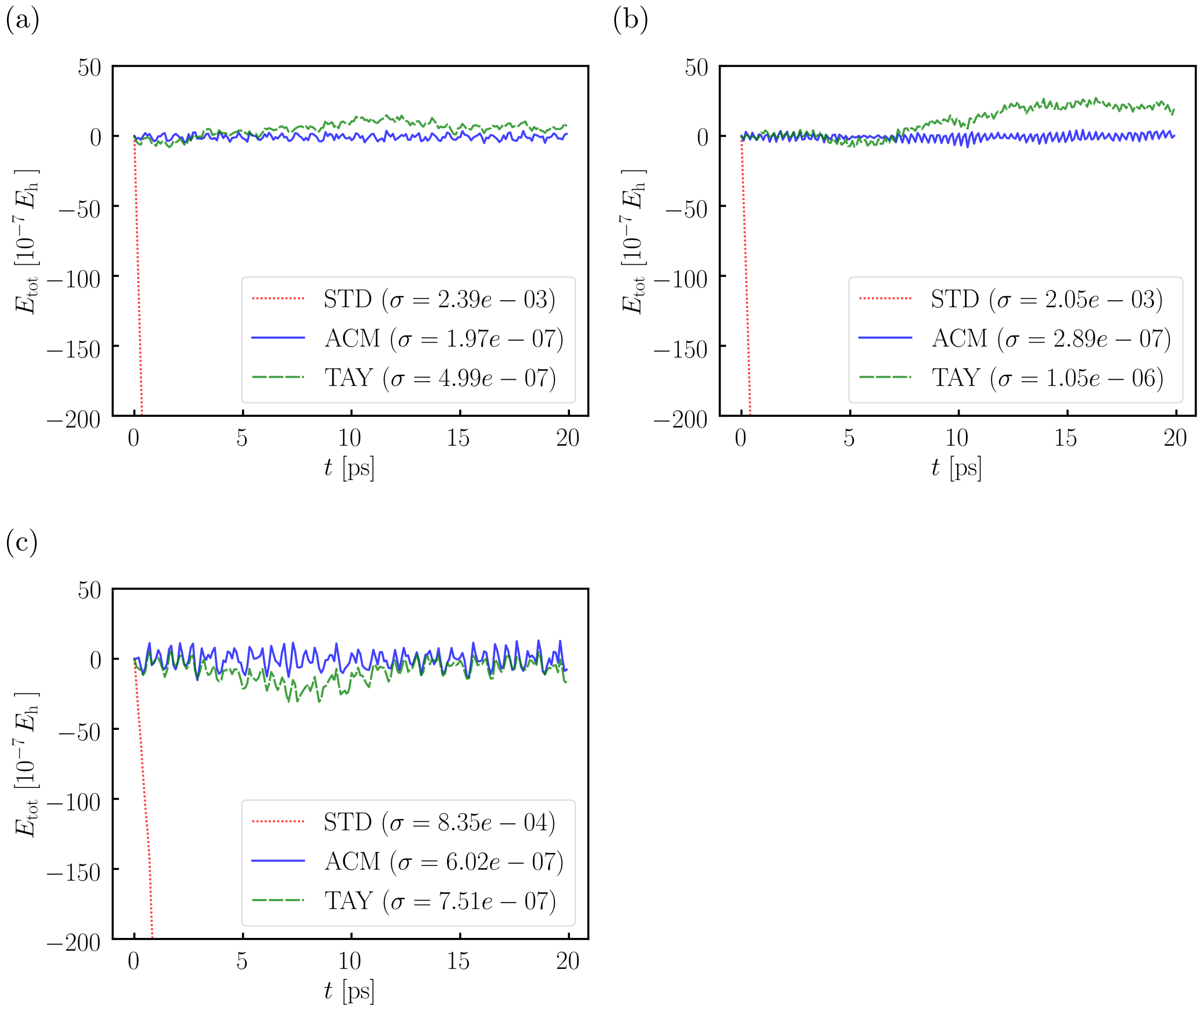


FIG. S4: Comparison of integration schemes for three trajectories (a-c) of $H_2$ (HF/cc-pVDZ level of theory, $\Delta t = 0.02\,\mathrm{fs}$, $T \approx 1000\,\mathrm{K}$) with $|\mathbf{B}| = 1.0\,B_0$: Velocity Verlet in its standard implementation (STD), auxiliary coordinates (ACM) and momenta form setting $\omega$ to 0.1, and Taylor expansion form (TAY). In all simulations, the Berry force was neglected. The standard deviation ($\sigma$) of the total energy ($E_{\mathrm{tot}}$) is also given.

## III. SCREENING OF $\omega$

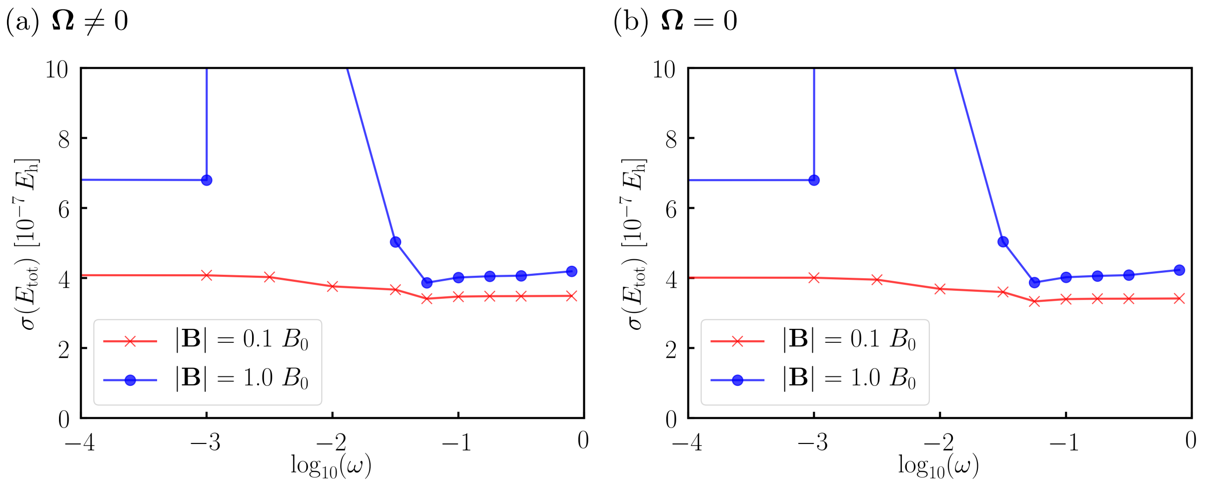


FIG. S5: Influence of $\omega$ on the stability of the dynamics of $H_2$ (HF/cc-pVDZ level of theory, velocity Verlet propagator, $\Delta t = 0.02\,\mathrm{fs}$, $T \approx 1000\,\mathrm{K}$, $N_{\mathrm{traj}} = 3$, and $t_{\mathrm{tot}} = 20\,\mathrm{ps}$) for $|\mathbf{B}| = 0.1\ B_0$ and $|\mathbf{B}| = 1.0\ B_0$ with (a) and without (b) Berry screening: Standard deviation ($\sigma$) of the total energy ($E_{\mathrm{tot}}$).

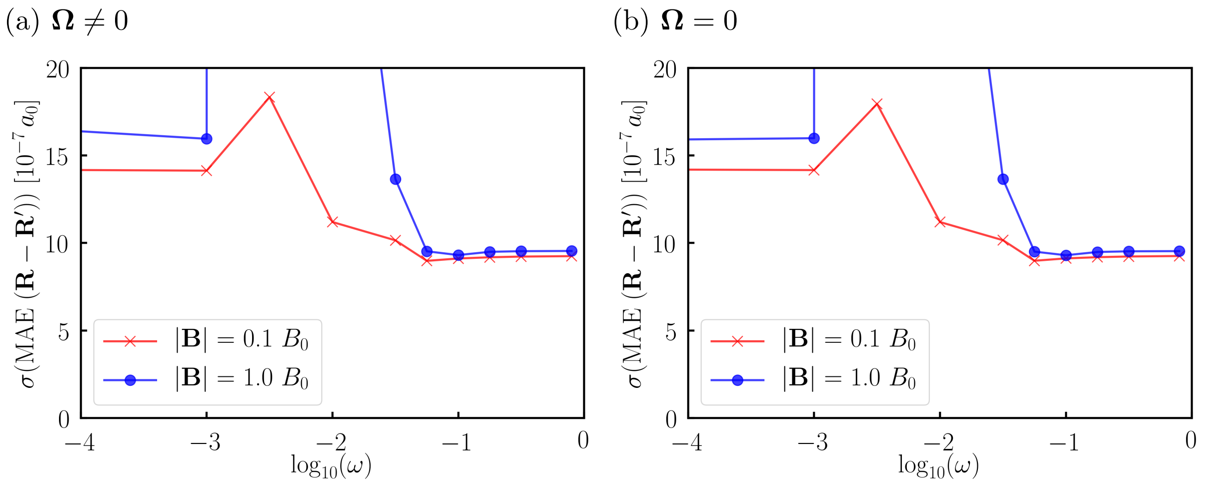


FIG. S6: Influence of $\omega$ on the stability of the dynamics of $H_2$ (HF/cc-pVDZ level of theory, velocity Verlet propagator, $\Delta t = 0.02\,\mathrm{fs}$, $T \approx 1000\,\mathrm{K}$, $N_{\mathrm{traj}} = 3$, and $t_{\mathrm{tot}} = 20\,\mathrm{ps}$) for $|\mathbf{B}| = 0.1\ B_0$ and $|\mathbf{B}| = 1.0\ B_0$ with (a) and without (b) Berry screening: Standard deviation ($\sigma$) of the mean absolute error of ($\mathbf{R}$ - $\mathbf{R}$').

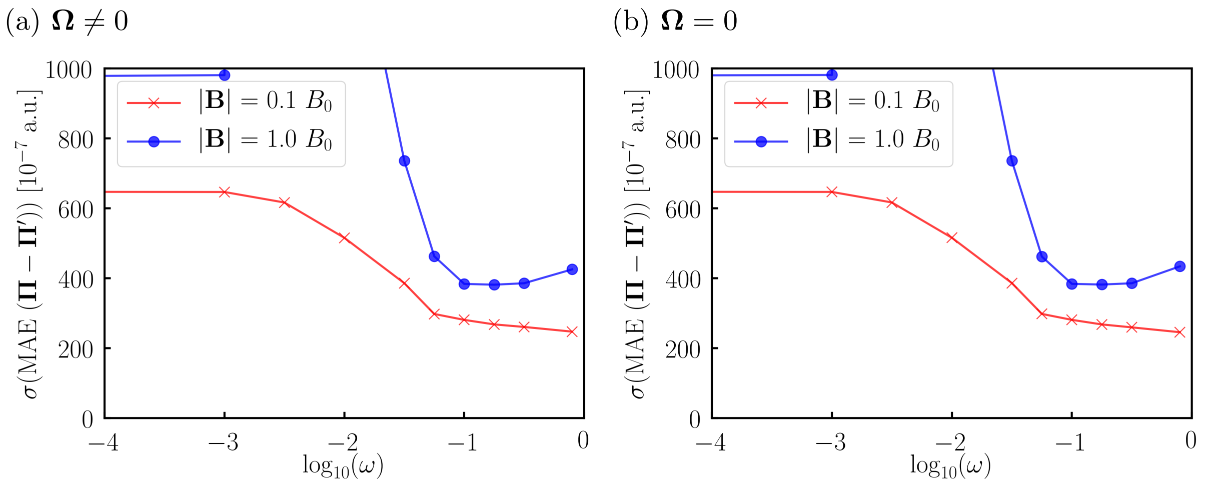


FIG. S7: Influence of $\omega$ on the stability of the dynamics of $H_2$ (HF/cc-pVDZ level of theory, velocity Verlet propagator, $\Delta t = 0.02\,\mathrm{fs}$, $T \approx 1000\,\mathrm{K}$, $N_{\mathrm{traj}} = 3$, and $t_{\mathrm{tot}} = 20\,\mathrm{ps}$) for $|\mathbf{B}| = 0.1\ B_0$ and $|\mathbf{B}| = 1.0\ B_0$ with (a) and without (b) Berry screening: Standard deviation ($\sigma$) of the mean absolute error of ($\mathbf{\Pi}$ - $\mathbf{\Pi}$').

## IV. SCREENING OF PROPAGATORS

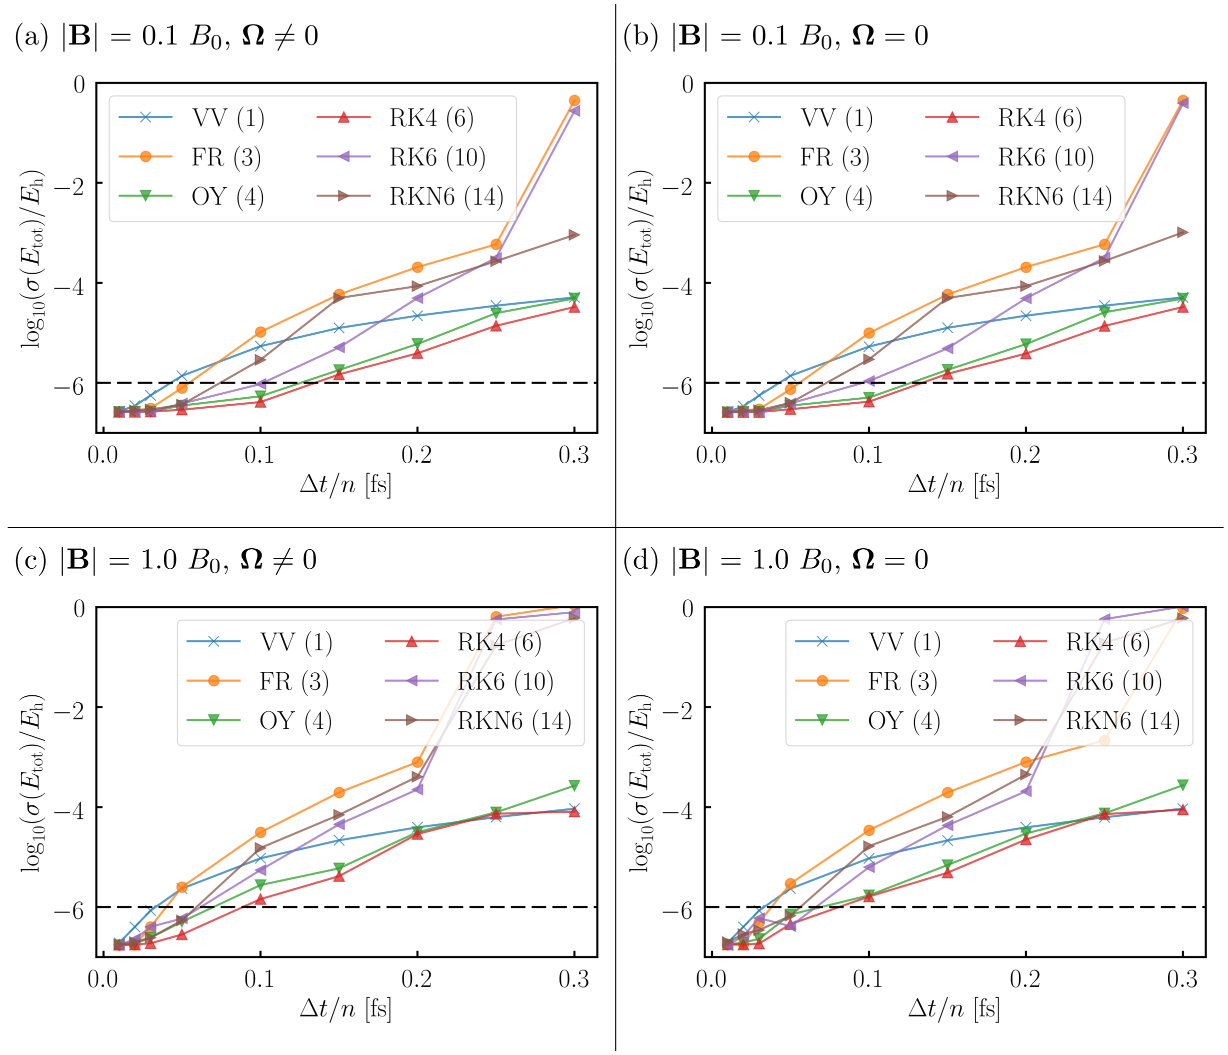


FIG. S8: Influence of the propagator (see Table S1) and the step size ($\Delta t$) on the stability of the dynamics of $H_2$ (HF/cc-pVDZ level of theory, $T \approx 1000\,\mathrm{K}$, $N_{\mathrm{traj}} = 3$, and $t_{\mathrm{tot}} = 20\,\mathrm{ps}$) for $|\mathbf{B}| = 0.1$ (a+b) and $|\mathbf{B}| = 1.0\,B_0$ (b+d) with (a+c) and without (b+d) Berry force: Standard deviation of the total energy ($\sigma(E_{\mathrm{tot}})$). The "optimal" $\omega$ with the lowest error is chosen out of $\omega = 10^{-1}$, $10^{-3}$, or $10^{-7}$ for every propagator-time step combination. $\Delta t$ is divided by the order ($n$) of the corresponding propagator (see legend) to yield the same computational cost. Our desired accuracy of $\sigma(E_{\mathrm{tot}}) = 10^{-6}\,E_{\mathrm{h}}$ is indicated by the dashed line.

## V. SCREENING OF $\omega$ AND PROPAGATORS

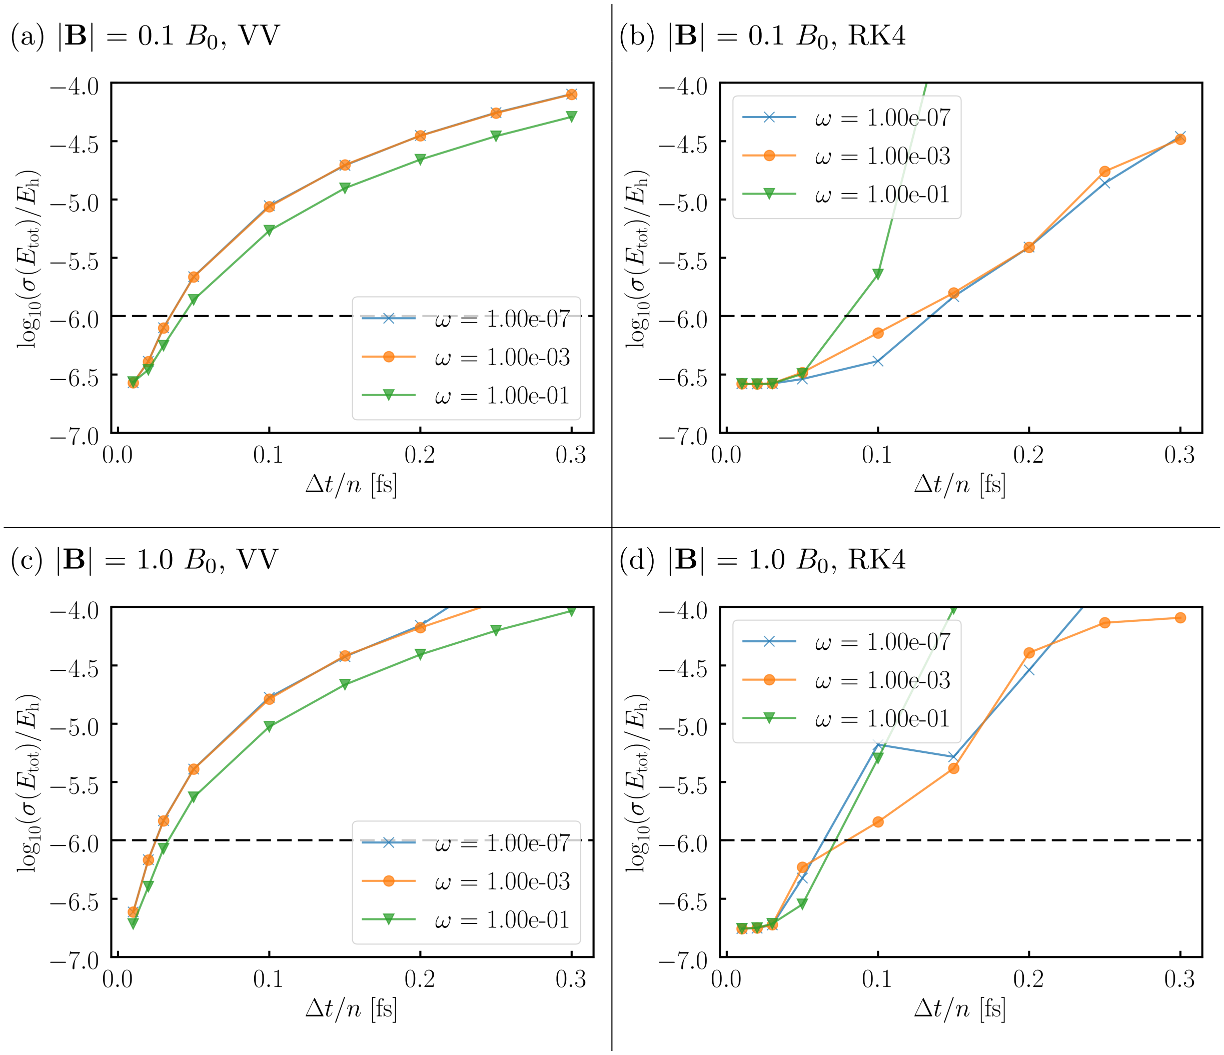


FIG. S9: Influence of $\omega$ and the step size ($\Delta t$) on the stability of the dynamics of $H_2$ (HF/cc-pVDZ level of theory, $T \approx 1000\,\mathrm{K}$, $N_{\mathrm{traj}} = 3$, and $t_{\mathrm{tot}} = 20\,\mathrm{ps}$) for $|\mathbf{B}| = 0.1\,B_0$ (a+b) and $|\mathbf{B}| = 1.0\,B_0$ (b+d) using the VV (a+c) and the RK4 (b+d) propagator (see Table S1): Standard deviation of the total energy ($\sigma(E_{\mathrm{tot}})$). All simulations were performed with Berry force. The time step $\Delta t$ is divided by the order ($n$) of the corresponding propagator ($n = 1$ for VV and $n = 6$ for RK4) to yield the same computational cost. Our desired accuracy of $\sigma(E_{\mathrm{tot}}) = 10^{-6}\,E_{\mathrm{h}}$ is indicated by the dashed line.

## VI. TRAJECTORIES AND "TRANSLATIONAL" SPECTRA OF HE

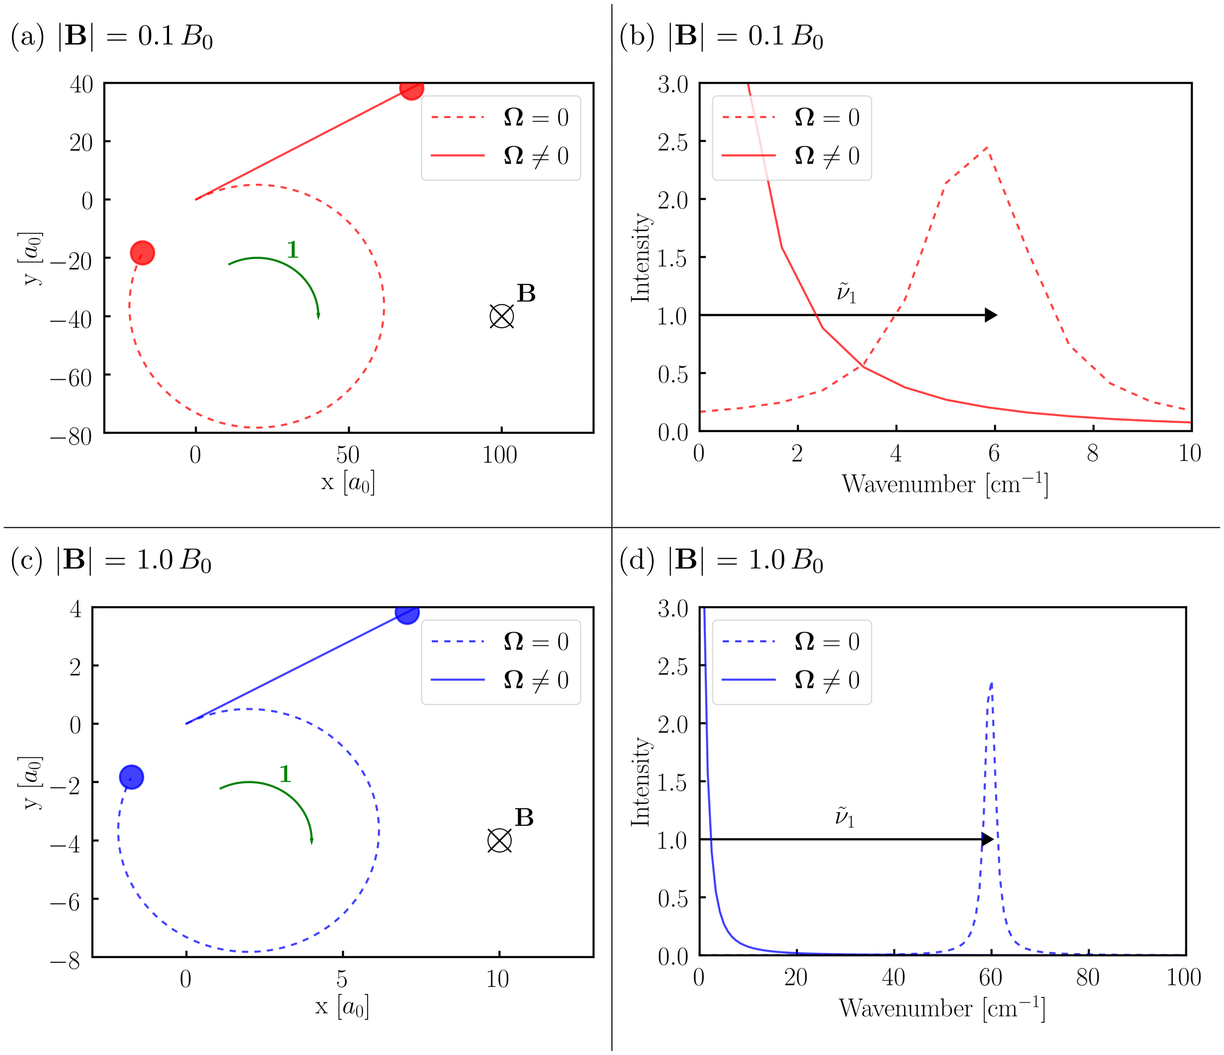


FIG. S10: Influence of the Berry screening ($\mathbf{\Omega}$) on the trajectory (a+c) and the resulting "translational" spectrum (b+d) of He simulated at $|\mathbf{B}| = 0.1\,B_0$ (a+b) and $|\mathbf{B}| = 1.0\,B_0$ (c+d) (HF/cc-pVDZ level of theory, ACM RK4 propagator, $\Delta t = 1\,\mathrm{fs}$, $T \approx 1000\,\mathrm{K}$, and $t_{\mathrm{tot}} = 20\,\mathrm{ps}$). The wavenumber $\tilde{\nu}_1$ in (b+d) corresponds to the cyclotron rotation that is indicated by the arrow in (a+c). Please note the different scale that is applied to the different magnetic field strengths.

## VII. TRAJECTORIES OF $H_2$

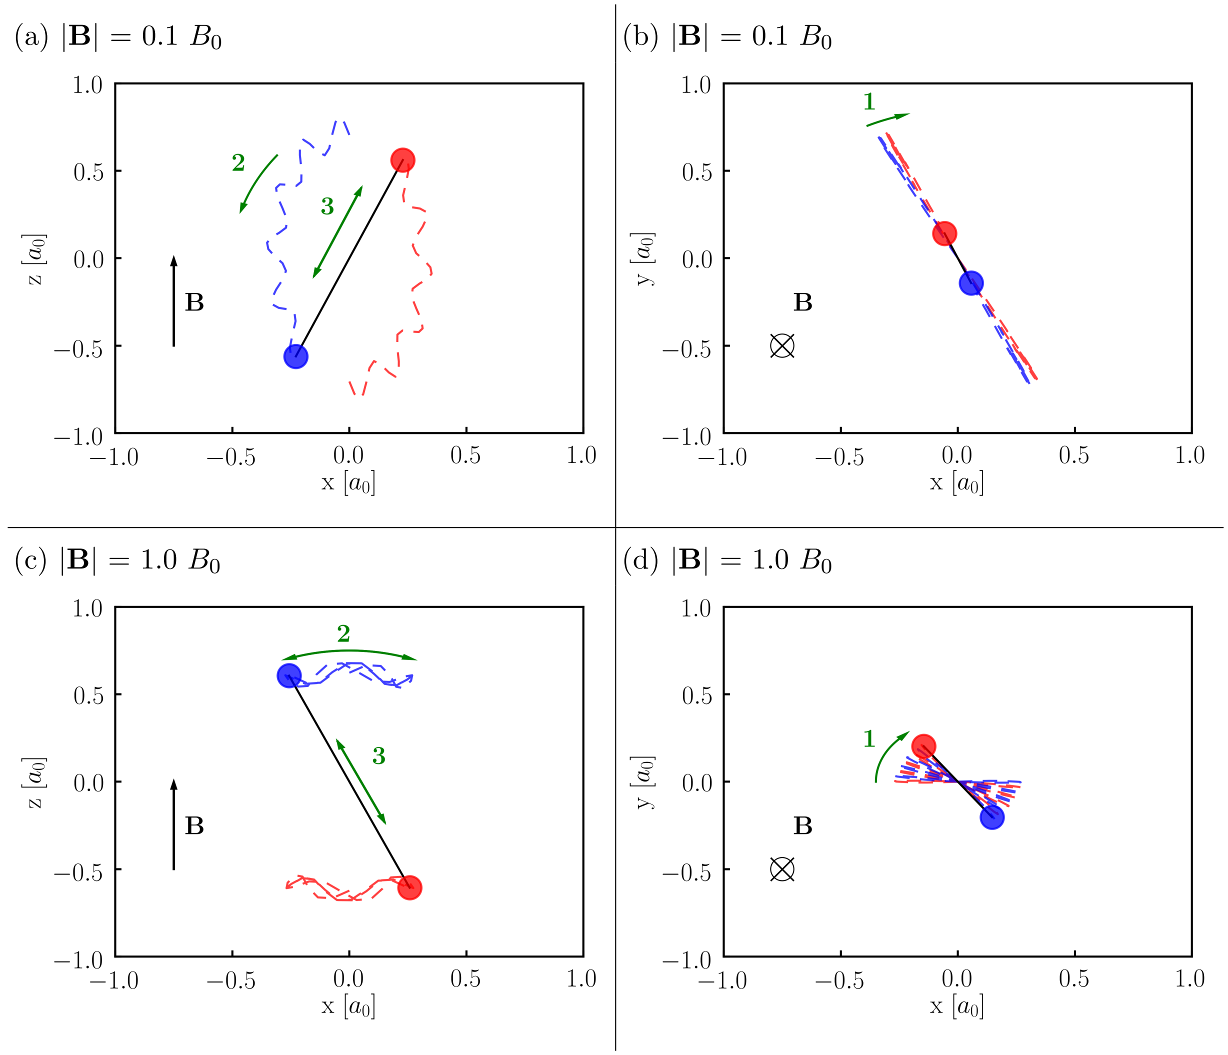


FIG. S11: Exempt of a trajectory of a molecular dynamics simulation of $H_2$ (HF/cc-pVDZ level of theory, ACM RK4 propagator, $T \approx 1000\,\mathrm{K}$) with $|\mathbf{B}| = 0.1\,B_0/\Delta t = 0.9\,\mathrm{fs}$ (a+b) and $1.0\,B_0/\Delta t = 0.6\,\mathrm{fs}$ (c+d). The magnetic field $\mathbf{B}$ is parallel to the $z$-axis with (a+c) showing the $xz$- and (b+d) showing the $xy$-plane. Both simulations were performed with Berry force. The green arrows/numbers indicate the three types of movement: (1) The cyclotron rotation, (2) the polar rotation/vibration, and (3) the H-H stretching vibration.

## VIII. ROVIBRATIONAL SPECTRA OF $H_2$

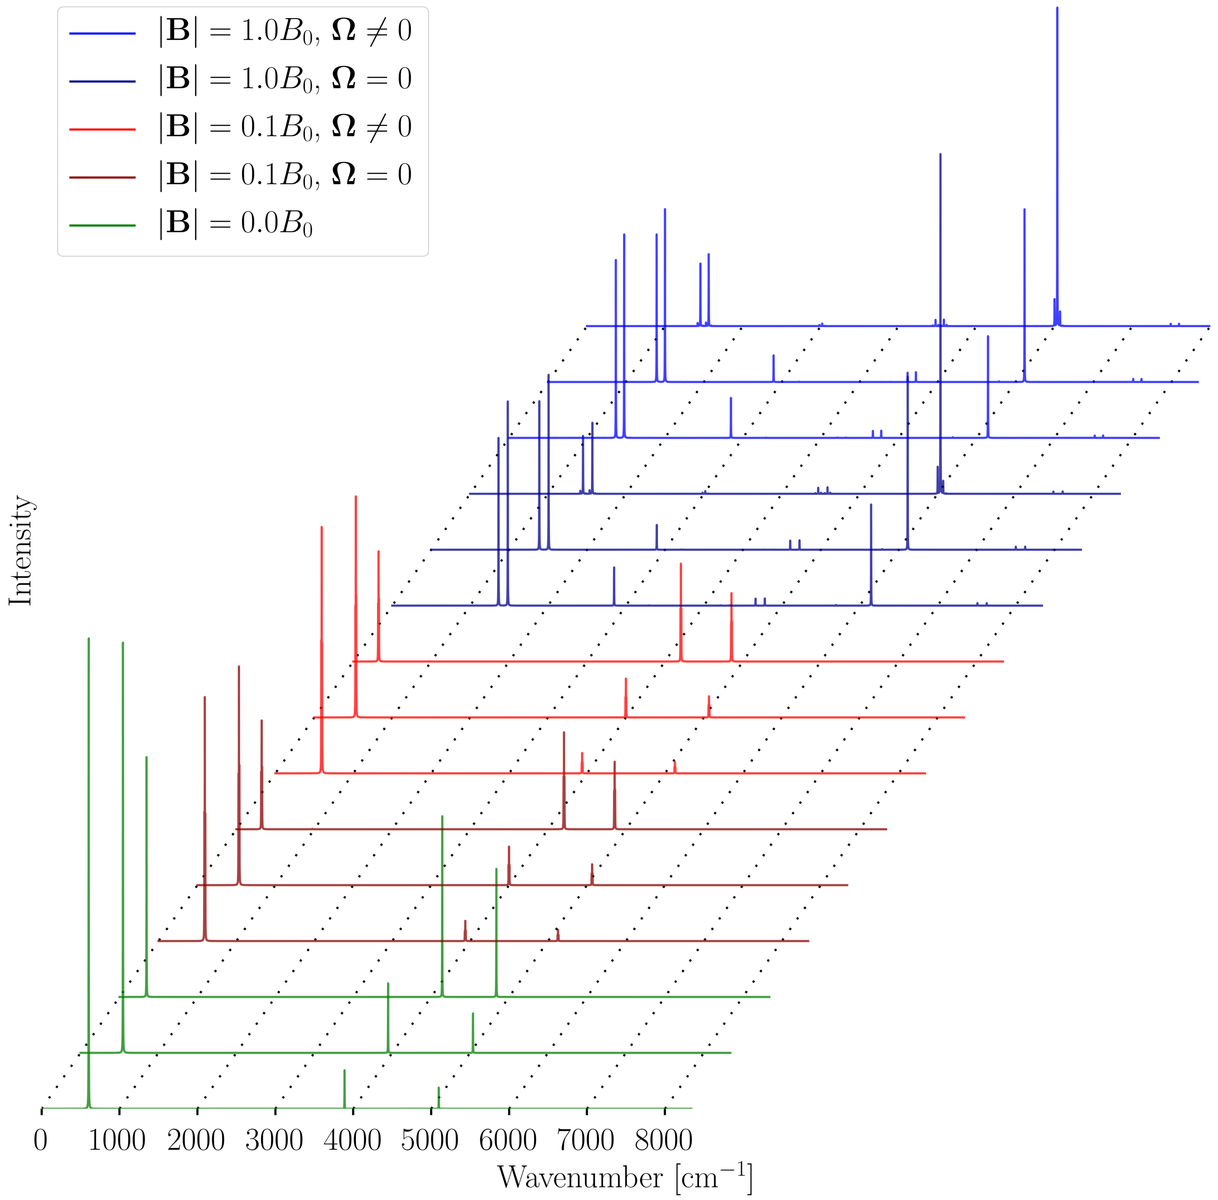


FIG. S12: Rovibrational spectra obtained from molecular dynamics simulations of $H_2$ (HF/cc-pVDZ level of theory, ACM RK4 propagator, $T \approx 1000\,\mathrm{K}$, and $t_{\mathrm{tot}} = 20\,\mathrm{ps}$) using three different initial momenta, different magnetic fields ($|\mathbf{B}| = 0.0$, 0.1, and $1.0\,B_0$), and simulations with and without Berry screening ($\mathbf{\Omega}$). In case of $|\mathbf{B}| = 0.0$, 0.1, and $1.0\,B_0$, a step size ($\Delta t$) of 1.0, 0.9, and 0.6 fs, respectively, was applied.

## IX. PSEUDOCODE FOR PROPAGATORS

Algorithm 1: General propagation scheme of (auxiliary) nuclear coordinates ($\mathbf{R}$, $\mathbf{R}'$) and momenta ($\boldsymbol{\Pi}$, $\boldsymbol{\Pi}'$) in the auxiliary coordinates and momenta (ACM) method for different orders ($n$). $\mathbf{F}$, $\Delta t$, $\mathbf{M}$, and $\boldsymbol{\omega}$ denote forces, step size, nuclear mass, and coupling frequency, respectively. The coefficients $a_i$ and $b_i$ for the different propagators and orders are listed in Table S1.

```
i = 0; a' = 0; b' = 0
while i ≤ n do
    Π = Π − Δt · a_i · F(R, Π')
    R' = R' + Δt · a_i · M^{-1} Π'
    a' = a' + a_i
    if i < n then
        Calculate F(R', Π)
        Π' = Π' − Δt · (a' − b') · F(R', Π)
        R = R + Δt · (a' − b') · M^{-1} Π
        b' = b' + b_i
        Apply Φ_ω(Δt · b_i)
        Calculate F(R', Π)
        Π' = Π' − Δt · (b' − a') · F(R', Π)
        R = R + Δt · (b' − a') · M^{-1} Π
        Calculate F(R, Π')
    end if
    i = i + 1
end while
```

## X. COEFFICIENTS FOR PROPAGATORS

TABLE S1: Coefficients $a$ and $b$ for the different integrators of order $n$.

| Integrator | Order ($n$) | Coefficients | |
|---|---|---|---|
| Velocity Verlet (VV) | 1 | $a_0$ = 0.5000000000000000 | $b_0$ = 1.0000000000000000 |
| Ref. 1 and 2 | | $a_1$ = 0.5000000000000000 | |
| Forest-Ruth (FR) | 3 | $a_0$ = 0.6756035959798289 | $b_0$ = 1.3512071919596578 |
| Ref. 3 | | $a_1$ = -0.1756035959798289 | $b_1$ = -1.7024143839193155 |
| | | $a_2$ = -0.1756035959798289 | $b_2$ = 1.3512071919596578 |
| | | $a_3$ = 0.6756035959798289 | |
| Omelyan (OY) | 4 | $a_0$ = 0.1786178958448091 | $b_0$ = 0.7123418310626054 |
| Ref. 4 | | $a_1$ = -0.0662645826698185 | $b_1$ = -0.2123418310626054 |
| | | $a_2$ = 0.7752933736500187 | $b_2$ = -0.2123418310626054 |
| | | $a_3$ = -0.0662645826698185 | $b_3$ = 0.7123418310626054 |
| | | $a_4$ = 0.1786178958448091 | |
| RK4 | 6 | $a_0$ = 0.0792036964311957 | $b_0$ = 0.2095151066133620 |
| $S_6$/O4 in ref. 5 | | $a_1$ = 0.3531729060497740 | $b_1$ = -0.1438517731798180 |
| | | $a_2$ = -0.0420650803577195 | $b_2$ = 0.4343366665664560 |
| | | $a_3$ = 0.2193769557534996 | $b_3$ = 0.4343366665664560 |
| | | $a_4$ = -0.0420650803577195 | $b_4$ = -0.1438517731798180 |
| | | $a_5$ = 0.3531729060497740 | $b_5$ = 0.2095151066133620 |
| | | $a_6$ = 0.0792036964311957 | |

| Integrator | Order ($n$) | Coefficients | |
|---|---|---|---|
| RK6 | 10 | $a_0$ = 0.0502627644003922 | $b_0$ = 0.1488164479010420 |
| $S_{10}$/O6 in ref. 5 | | $a_1$ = 0.4135143004283440 | $b_1$ = -0.1323858657677840 |
| | | $a_2$ = 0.0450798897943977 | $b_2$ = 0.0673076046921850 |
| | | $a_3$ = -0.1880548538195690 | $b_3$ = 0.4326664025781750 |
| | | $a_4$ = 0.5419606784507800 | $b_4$ = -0.0164045894036180 |
| | | $a_5$ = -0.7255255585086897 | $b_5$ = -0.0164045894036180 |
| | | $a_6$ = 0.5419606784507800 | $b_6$ = 0.4326664025781750 |
| | | $a_7$ = -0.1880548538195690 | $b_7$ = 0.0673076046921850 |
| | | $a_8$ = 0.0450798897943977 | $b_8$ = -0.1323858657677840 |
| | | $a_9$ = 0.4135143004283440 | $b_9$ = 0.1488164479010420 |
| | | $a_{10}$ = 0.0502627644003922 | |
| RKN6 | 14 | $a_0$ = 0.0378593198406116 | $b_0$ = 0.0917191526244616 |
| $SRKN^a_{14}$/O14-6 in ref. 5 | | $a_1$ = 0.1026356331024350 | $b_1$ = 0.1839831700050060 |
| | | $a_2$ = -0.0258678882665587 | $b_2$ = -0.0565343658328883 |
| | | $a_3$ = 0.3142414030714470 | $b_3$ = 0.0049146887747129 |
| | | $a_4$ = -0.1301444595174150 | $b_4$ = 0.1437611271683580 |
| | | $a_5$ = 0.1064177003695430 | $b_5$ = 0.3285676937468040 |
| | | $a_6$ = -0.0087942431285106 | $b_6$ = -0.1964114664864542 |
| | | $a_7$ = 0.2073050690568954 | $b_7$ = -0.1964114664864542 |
| | | $a_8$ = -0.0087942431285106 | $b_8$ = 0.3285676937468040 |
| | | $a_9$ = 0.1064177003695430 | $b_9$ = 0.1437611271683580 |
| | | $a_{10}$ = -0.1301444595174150 | $b_{10}$ = 0.0049146887747129 |
| | | $a_{11}$ = 0.3142414030714470 | $b_{11}$ = -0.0565343658328883 |
| | | $a_{12}$ = -0.0258678882665587 | $b_{12}$ = 0.1839831700050060 |
| | | $a_{13}$ = 0.1026356331024350 | $b_{13}$ = 0.0917191526244616 |
| | | $a_{14}$ = 0.0378593198406116 | |

## REFERENCES

[1]L. Verlet, Phys. Rev. **159**, 98 (1967).

[2]W. C. Swope, H. C. Andersen, P. H. Berens, and K. R. Wilson, J. Chem. Phys. **76**, 637 (1982).

[3]E. Forest and R. D. Ruth, Phys. D **43**, 105 (1990).

[4]I. P. Omelyan, I. M. Mryglod, and R. Folk, Comput. Phys. Commun. **151**, 272 (2003).

[5]S. Blanes and P. C. Moan, J. Comput. Appl. Math. **142**, 313 (2002).
